# Supplementary material for: An off-the-grid approach to multi-compartment magnetic resonance fingerprinting
Source: arXiv:2011.11193 source file (2020-11-23)
Supplement: Supplementary file 1 [file supp_theory.tex]

% !TEX root = ../offgridQMRI.tex

\newcommand{\JJ}{\mathbb{J}}
\newcommand{\HH}{\mathbb{H}}

\section{Support stability}

\paragraph{Notations}
 For $\phi:\RR^d \to \RR^T$, let $\JJ_\phi(\theta) \in \RR^{T\times d}$ denote the Jacobian of $\phi$ at $\theta$.   Given a matrix $Q\in \RR^{n\times m}$, let $\vc_{n,m}(p)\in\RR^{nm}$ be its vectorized version with columns stacked vertically, let $\rc_{n,m}$ be the inverse operation, so that $\rc_{n,m}(\vc_{n,m}(p)) = p$. Finally, we define the soft-thresholding operator by $S_\beta:\RR^v \to \RR^v$ is defined by  $$S_\beta(\xi)_i = \begin{cases} \xi_i -\beta &\xi_i >\beta,
\\ \xi_i +\beta &\xi_i<-\beta,
 \\0  & \abs{\xi_i}\leq \beta.
\end{cases}.$$
Given a matrix or a tensor, we write  $\norm{\cdot}$ without subscript to denote the operator norm with respect to the vector norm $\norm{\cdot}_2$. Given an index set $I$ and a vector $V$, we denote by $\proj_I(V)$ the restriction of $V$ to the index set $I$. Given a point $x\in \RR^n$ and $r>0$, we denote by $\Bb(x,r) \eqdef \enscond{z}{\norm{x-z}<r}$ the open ball of radius $r$ around $x$.

\subsection{The precertificate as a least squares solution}\label{supp:precertificate_lsq}
We detail here how to write the solution of $Q_\btheta$ as the solution of a linear system. Observe that the constraints $\proj_{I_s}f(\theta_s) = \frac{\proj_{I_s}C_s}{\norm{C_s}_2}$ for all $s\in [k]$ can be written as
\begin{align*}
\proj_{\bold{I}} \vc_{k,v} \pa{ \Phi^\top_{\btheta} Q}= \proj_{\bold{I}} [\Id_v \otimes D_{\btheta}^\top]\vc_{T,v}(P) = u_0
\end{align*}
where $u_0 = \pa{(1-\beta) +\beta  \sqrt{v}\proj_{I_s}  C_s/\norm{C_s}_2}_{s=1}^k \in \RR^{\sum_s \abs{I_s}}$ and 
$\proj_{\bold{I}}: \RR^{kv} \to \RR^{\sum_s \abs{I_s}}$ is the  subsampling operator given  by which selects the nonzero entries of $\ens{I_s}_{s\in[k]}$, so that given a matrix $z \in \RR^{k\times v}$ with $s^{th}$ row $z_s \in \RR^{v}$ for $s\in [k]$, $\proj_{\bold{I}} \vc(z) = \pa{(z_s)_{I_s}}_{s\in [k]}$.

The constraints $\partial_\theta \norm{f(\theta_s)}_2^2 = 0$  for all $s\in [k]$ can be written as
\begin{align*}
\mathbf{0}_d &= \beta \sqrt{v} \sum_{i\in I_s}  f_i(\theta_s) \nabla f_i(\theta_s)  = \frac{1}{\norm{C_s}_2} \sum_{i=1}^v (C_s)_i \nabla [\Phi^* Q](\theta_s) \\
&= \JJ_\phi(\theta_s)^\top Q \frac{C_s}{\norm{C_s}_2} =\frac{1}{\norm{C_s}_2}[ C_s^\top\otimes \JJ_\phi(\theta_s)^\top]\vc_{T,v}(P)
\end{align*}

We can therefore define the $Tv\times (\sum_{s=1}^k \abs{I_s}+kd)$ matrix \begin{equation}\label{eq:Gamma}
\Gamma = \left[(\Id_v\otimes D_\btheta ) \proj_{\bold{I}}^* ,\frac{ C_1}{\norm{C_1}_2} \otimes \JJ_\phi(\theta_1), \cdots, ,\frac{ C_k}{\norm{C_k}_2} \otimes \JJ_\phi(\theta_k) \right]
 \end{equation}
 and write
 $$Q_\btheta = \rc_{T,v} \pa{(\Gamma^*)^\dagger \begin{pmatrix}
u_0\\
\mathbf{0}_{kd}
\end{pmatrix}}.$$ Note that $\Gamma$ depends on $\btheta$ and $\ens{C_s/\norm{C_s}_2}_s$. To make this dependence clear, we will sometimes write $\Gamma_{\btheta,C}$ in place of $\Gamma$.

\subsection{The dual of sparse group Blasso}

The proof of Theorem \ref{thm:stability} is via analysis of the dual problem to \eqref{eq:spglasso}.  The proof follows closely the proof of support stability from \cite{duval2015exact}, however, we present the details here since the case of vector-valued measured with the sparse group norm has not be covered in the literature. 
We describe the some primal dual relationships in this section.

To simplify notation, throughout this section and the next, we let  $\lambda_1 \eqdef \beta$ and $\lambda_2 \eqdef \sqrt{v}(1-\beta)$.

\paragraph{Duality for sparse group lasso}
Before describing the dual problem, we first mention a duality, described in~\footnote{O.~Burdakov and B.~Merkulov, ``On a new norm for data fitting and optimization
  problems,'' \emph{Link{\"o}ping University, Tech. Rep.
  LiTH-MAT}, 2001.}, % \cite{burdakov2001new}, 
  between the vector norm (for $x\in\RR^n$ and $\epsilon>0$), $J(x) \eqdef  \epsilon \norm{x}_1 + (1-\epsilon)\norm{x}_2$, and the so-called $\epsilon$-norm, which is defined for $\xi\in\RR^n$ as  $\nu = \norm{\xi}_\epsilon$  is the unique $\nu>0$ such that
$$
\sum_i (\abs{\xi_i} - (1-\epsilon)\nu)_+^2 - (\epsilon \nu)^2 = 0.
$$
It is shown in~\footnote{E.~Ndiaye, O.~Fercoq, A.~Gramfort, and J.~Salmon, ``Gap safe screening rules
  for sparse-group lasso,'' in \emph{Advances in neural information processing
  systems}, 2016, pp. 388--396.} Appendix E, Lemmas 1 and 2 (see also~$^4$) that \footnote{which of course can be written as: for all $\lambda_1,\lambda_2>0$, \begin{equation*}
\begin{split}
&\enscond{x+y}{\norm{x}_2 \leq \lambda_1 \nu, \norm{y}_\infty \leq\lambda_2 \nu} = \enscond{\xi}{  \norm{S_{\lambda_2}(\xi)}^2_2 \leq  (\lambda_1 \nu)^2 }
\end{split}
\end{equation*}}
\begin{equation}\label{eq:epsnorm1}
\begin{split}
&\enscond{x+y}{x,y\in\RR^d, \norm{x}_2 \leq \epsilon \nu, \norm{y}_\infty \leq (1-\epsilon) \nu} \\
&= \enscond{\xi\in \RR^d}{\norm{\xi}_\epsilon \leq \nu}
\end{split}
\end{equation}
and hence, the dual norm of $J$ is the $\epsilon$-norm. Moreover, we have the \emph{unique} $\epsilon$-decomposition
$$
\xi = S_\epsilon(\xi) + (\xi - S_\epsilon(\xi) )
$$
with $\norm{S_\epsilon(\xi)}_2 = (1-\epsilon) \norm{\xi}_\epsilon$ and $\norm{\xi - S_\epsilon(\xi) }_\infty = \epsilon\norm{\xi}_\epsilon$,
where we recall that $S_\epsilon$ is the soft-thresholding operator.

 \paragraph{The dual of sparse group Blasso}
 \begin{lem}\label{lem:pd}
 The dual problem to \eqref{eq:spglasso} is
 \eql{\label{eq:spglassodual}
\sup_{Q \in K} \dotp{X}{Q}_F - \alpha \norm{Q}_F^2 \tag{$\Dd_\al(X)$}
}
where $\Kk \subseteq \RR^{T\times v}$ is defined as
$$
\Kk  \eqdef 
\enscond{Q}{\eta \eqdef \Phi^* Q, \; \sum_{i=1}^v ({\eta_i(\theta)} - \lambda_1 )_+^2 \leq \lambda_2^2}
 $$
 The primal and dual problems are related by $\meas$ solves \eqref{eq:spglasso} if and only if $Q= \frac{X-\Phi \meas }{\alpha}$ solves \eqref{eq:spglassodual}.  Moreover, $\Phi^* Q \in \partial \norm{\meas}_\beta$.
 \end{lem}
\begin{proof}
By considering the dual norms of $\abs{\meas}_1$ and $\abs{\meas}_2$, it holds
\begin{equation}\label{eq:eps_decomp}
\begin{split}
&\norm{\meas}_\beta =  \sup_{\sup_\theta\norm{f(\theta)}_\infty \leq \beta} \dotp{f}{\meas} +  \sup_{\sup_\theta\norm{g(\theta)}_2  \leq \la_2} \dotp{g}{\meas}\\
&= \sup \enscond{ \dotp{f+g}{\meas} }{ \forall \theta, \; \norm{f(\theta)}_\infty \leq \la_1, \norm{g(\theta)}_2 \leq \la_2}
\end{split}
\end{equation}

%It is known from \cite{} that  for $\epsilon>0$,
%\begin{align*}
%&\enscond{x+y}{x,y\in\RR^d, \norm{x}_2 \leq \epsilon \nu, \norm{y}_\infty \leq (1-\epsilon) \nu} \\
%&= \enscond{\xi\in \RR^d}{\norm{\xi}_\epsilon \leq \nu}
%\end{align*}
%where the so-called $\epsilon$-norm, defined as $\nu = \norm{\xi}_\epsilon$  is the unique $\nu>0$ such that
%$$
%\sum_i (\abs{\xi_i} - (1-\epsilon)\nu)_+^2 - (\epsilon \nu)^2 = 0.
%$$
%Therefore,
From \eqref{eq:epsnorm1}, 
\begin{align*}
&\enscond{x+y\in\RR^d}{ \norm{x}_2 \leq \la_2 , \norm{y}_\infty \leq  \la_1 } \\
&= \enscond{\xi\in \RR^d}{ \norm{S_{\la_1}(\xi)}_2^2 \leq \la_2 }
\end{align*}
and
$
\norm{\meas}_{\beta} = 
\sup_{f\in\Kk_0}{\dotp{f}{\meas}}
$
where $$\Kk_0 = \enscond{ f\in \Cc(\Tspace;\RR^v)}{  \sup_{\theta\in\Tspace}   \norm{S_{\la_1}( f(\theta))}_2^2 \leq \la_2^2}.
$$
Note that we can restrict the set $\Kk_0$ to positive functions $\Kk_+ \eqdef \Kk_0 \cap \Cc(\Tspace;\RR_+^v)$ since $\meas$ is a positive measure.
Therefore, the convex conjugate of $J(\meas) \eqdef \norm{\meas}_\beta$ is $\iota_{\Kk_+}$, the indicator function on the set $\Kk_+$.

The result now follows by applying the Fenchel-Rockafellar duality Theorem 4.2\footnote{I.~Ekeland and R.~Temam, \emph{Convex analysis and variational problems}.\hskip
  1em plus 0.5em minus 0.4em\relax SIAM, 1999.}.  %\cite[Thm 4.2]{ekeland1999convex}.

\end{proof}

Given a dual solution $Q_\alpha$ to \eqref{eq:spglassodual}, the function  $f(\theta) \eqdef \frac{1}{\la_2  }  (\eta(\theta) - \la_1)_+$ with $\eta \eqdef \Phi^* Q_\alpha$ characterizes the support of any primal solution $\meas_\alpha$ of \eqref{eq:spglasso} in the following sense:

\begin{lem}\label{lem:structure}
Any solution $\meas_\alpha$ to \eqref{eq:spglassodual} satisfies
$$
\Supp(\meas_\alpha) \subseteq \enscond{\theta\in\Tspace}{ \norm{f(\theta)} = 1  }.
$$
 If  $\meas_\alpha = \sum_s C_s^\top \delta(\theta - \theta_s)$ is a discrete measure, then for each $s$, $\Supp(C_s) \subseteq \enscond{j \in [v]}{\eta_j(\theta_s) > \la_1}$ and $f(\theta_s) = C_s/\norm{C_s}_2$.
 
 \end{lem}
\begin{proof}

We know $\eta = \Phi^* p \in \partial \abs{\meas}_\beta = \la_1 \partial \abs{\meas}_1  + \la_2 \abs{\meas}_2$.
From
\eqref{eq:eps_decomp}, if $\xi$ satisfies $\sum_i ( \xi - \la_1)_+^2 \leq \la_2^2$
then $\norm{S_{\la_1}(\xi)}_2 \leq \la_2$ and  $\norm{\xi - S_{\la_1}(\xi)}_\infty \leq \la_1$. So $S_{\la_1}(\eta) \in \la_2 \partial \abs{\meas}_2$ which gives the first inclusion. For the second,
$$
\eta - S_{\la_1} (\eta) \in \la_1 \partial \abs{\meas}_1
$$
which means that given $s\in [k]$ and $I_s = \Supp(C_s)$,
$$
\proj_{I_s } \pa{\eta(\theta_s) - \max(\eta(\theta_s) - \la_1 ,0) } = \la_1 \proj_{I_s} \sign(C_s)
$$
If  $ \eta(\theta_s)_j < \la_1 $ for $j\in I_s$, then this equation implies that $\eta(\theta_s)_j = \la_1 \sign(C_s)_j$ which is a contradiction. Therefore, $I_s \subset \enscond{j}{\eta_j(\theta_s)>\la_1}$.

\end{proof}

Note that \eqref{eq:spglassodual} has a unique solution, since it can be seen as the projection of $X/\alpha$ onto the closed convex set $K$.  Moreover, the previous lemma shows that its solution characterises the support of any primal solution $\meas$ of \eqref{eq:spglasso}. Therefore, to understand the structure of solutions to \eqref{eq:spglasso} with   $X = \Phi \meas + w$ with $\norm{w}\leq \epsilon$, it suffices to study the solution of the dual problem \eqref{eq:spglassodual}, which we denote by $Q_{\alpha,\epsilon}$.
%\begin{lem}
%Let $Q_\alpha$ solve \eqref{eq:spglassodual}. Then, letting $\eta_\alpha \eqdef \Phi^* p_\alpha$, any solution $\meas_\alpha$ to \eqref{eq:spglassodual} satisfies
%$$
%\Supp(\meas_\alpha) \subseteq \enscond{\theta\in\Tspace}{ \sum_i (\eta_i(\theta) - \beta)_+^2 =v (1-\beta)^2  }
%$$
% and if $\meas_\alpha = \sum_s C_s^\top \delta(\theta - \theta_s)$ is a discrete measure, then for each $s$, $\Supp(C_s) \subseteq \enscond{j \in [v]}{\eta_j(\theta_s) > \beta}$.
%\end{lem}
Following \cite{duval2015exact}, we can show that $Q_{\alpha,\epsilon}$ has a limit as $\epsilon/\alpha$ and $\alpha$ converge to 0:
Define the \textit{minimal norm certificate} by
\begin{equation}
\begin{split}
Q_0 \in \argmin \enscond{\norm{Q}_F}{\eta \eqdef \Phi^* Q \in \Kk, \; \dotp{\eta}{\meas} = \norm{\meas}_\beta}.
\end{split}
\end{equation}
\begin{lem}
We have $\norm{Q_{\alpha,0} - Q_0}_F \to 0$ as $\alpha\to 0$, and
$$
\norm{Q_{\alpha,\epsilon} - Q_{\alpha, 0}}_F \leq \epsilon/\alpha.
$$
\end{lem}
\begin{proof}
The proof is omitted as it is verbatim the proof of Proposition \todo{}\ref{} in \cite{duval2015exact}
\end{proof}

\begin{rem}
The minimal norm certificate $Q_0$ is  a solution to the dual problem \eqref{eq:spglassodual} with $\alpha = 0$ and $X = \Phi \meas$. Moreover, from Lemma \ref{lem:structure}, for a discrete measure $\meas = \sum_s C_s^\top \delta(\theta-\theta_s)$, we in fact have, writing $f_Q \eqdef\frac{1}{\la_2}(\Phi^* Q - \la_1)_+$,
\begin{equation}
\begin{split}
Q_0 \in \argmin \enscond{\norm{Q}_F}{  \sup_{\theta\in\Tspace} \norm{f_Q(\theta)}_2 \leq 1 \;f_Q(\theta_s) = \frac{C_s}{\norm{C_s}_2}}.
\end{split}
\end{equation}
\end{rem}

Define $\eta_0 \eqdef \Phi^* Q_0$  and $f_0 \eqdef \frac{1}{\la_2} (\eta_0 -\la_1)_+$.
We say that $Q_0$ is nondegenerate  with respect to a sparse measure $\mestar = \sum_{s=1}^k C_s \delta(\theta - \theta_s)$ 
if it satisfies 
\begin{enumerate}
\item $\norm{f_0(\theta)}_2<1$ for all $\theta\not\in \ens{\theta_i}$
\item for each $s\in [k]$, $f_0(\theta_s) =  \frac{C_s}{\norm{C_s}_2}$.
\item  letting $g(\theta) \eqdef  \norm{f_0(\theta)}_2^2$, $g''(\theta_s) \neq 0$ for all $s\in [k]$. 
%and 
%$$
%\sum_{i\in \Supp(C_s)} ({\eta_i(\theta_s)} - \beta )_+\nabla^2 \eta_i(\theta) +\nabla \eta_i(\theta_s) [\nabla \eta_i(\theta_s) ]^\top <0
%$$
\end{enumerate}

\begin{prop}\label{prop:stability}
If $Q_0$ is nondegenerate, then provided that $\epsilon/\alpha$ and $\alpha$ are sufficiently small, the solution to \eqref{eq:spglasso} is of the form $\meas_{\alpha,\epsilon} = \sum_{j=1}^k \hat C_j \delta(\theta-\hat \theta_j)$ where $\Supp(\hat C_j) \subseteq \Supp(C_j)$.
\end{prop}
\begin{proof}
From \eqref{eq:spglassodual}, we see that the dual solution to \eqref{eq:spglassodual} can be written as the projection of $X/\alpha$ onto the set $\Kk$. 
So, from $\norm{Q_{\alpha,\epsilon}-Q_{\alpha,0}} \leq  \norm{\proj_\Kk(X/\alpha) - \proj_\Kk((X+w)/\alpha)}  \leq \norm{w}_F/\alpha$, we have that $\eta_{\al,\epsilon} \eqdef \Phi^* Q_{\al,\epsilon} \to \eta_0$ in the uniform norm as $\alpha$ and $\epsilon/\alpha$ converge to 0. So, if $\eta_0$ is non-degenerate, then given any $r>0$, provided that $\norm{w}_F/\alpha$ and $\alpha$ are sufficiently small, letting $g(\theta) \eqdef \frac{1}{\la_2^2} \norm{(\eta_{\al,\epsilon}(\theta) - \la_1)_+}^2 $, we have $g(\theta)<1$ for all $\theta \not\in  \cup_j \Bb(\theta_j,r)$, and for all $\theta\in \Bb(\theta_j,r)$, $g''(\theta) \neq 0$. So, there are at most $k$ points for which $g(\theta) = 1$.  So, by Lemma \ref{lem:structure}, given data $X =\Phi \meas + w$, we recover at most $k$ components with $\meas_{\alpha,\epsilon} = \sum_{j=1}^k \hat C_j \delta(\theta-\hat \theta_j)$. Finally, uniform convergence of $\eta_{\alpha,\epsilon}$  to $\eta_0$ also ensures that $\Supp(\hat C_j) \subseteq \Supp(C_j)$ for $\alpha$ and $\epsilon/\alpha$ sufficiently small.
\end{proof}

To establish support stability, it suffices to show that $Q_0$ is nondegenerate. 
In general, $Q_0$ does not have a closed form expression and can be hard to compute, and in practice, one computes the precertificate $Q_V$ instead: Notice that
since $\norm{f_0(\theta)}^2 \leq 1$ for all $\theta$ and $\norm{f_0(\theta_s)}_2 = 1$, it is necessary that $\partial_\theta \norm{f_0(\theta_s)}_2^2 = 0$  for all $s\in [k]$. Hence, if we add the constraint that $\sup_\theta \norm{ f_p(\theta)}\leq 1$ to the constraint set in the definition of the vanishing derivatives precertificate $\eta_V$, then we have $\eta_V = \eta_0$. In other words, if  $\sup_\theta \norm{ f_V(\theta)}\leq 1$, then we must have $\eta_V = \eta_0$, and moreover, nondegeneracy of $\eta_V$ implies  that $\eta_0 = \eta_V$ is also nondegenerate.

\subsection{A quantitative result on support stability}\label{supp:theory_proof}

To prove Theorem \ref{thm:stability}, we rely on the implicit function theorem. The classical implicit function theorem is as follows:
\begin{prop}[Implicit function theorem]\label{prop:IFT}
Let $u_0\in\RR^m$, $v_0\in \RR^n$.
Let $f: \RR^{m} \times \RR^{n}\to \RR^n$ be such that $f(u_0, v_0) = 0$ and $\partial_u f(u_0,v_0)$ is invertible. Then, there exists a neighbourhood $V$ of $v_0$ and a neighbourhood $U$ of $u_0$, and a continuously differentiable function $g:V\to U$ such that 
$$
f(u,v) = 0 \iff u = g(v).
$$
Moreover, for all $v\in V$, the Jacobian of $g$ is $$J_g(v)  =\pa{ \partial_u f(g(v), v)}^{-1} \partial_v f(g(v), v).$$

\end{prop}

Typical quantitative versions of the implicit function theorem require showing invertibility  of $\partial_u f(u,v)$  and obtaining norm bounds on the partial derivatives of $f$  in some neighbourhood of $U$ of $u_0$ and $V$ of $v_0$. A quantitative version is proved in \cite[Section 4.3]{}, which requires to look at $\partial_u f(u,v)$  only when $f(u,v) = 0$. We present their arguments below and restate their result in greater generality.  
\begin{prop} \label{prop:IFT_quant}
Let $U_0$ be an open neighbourhood of $u_0$.
Let $R_2>0$. Assume that for all $u\in U_0$ and $v\in \Bb(v_0,R)$, $f(u,v) = 0$ implies that $\partial_u f(u,v)$ is invertible and  $\norm{\partial_u f(u,v)^{-1} \partial_v f(u,v)} \leq M$. Let $r_0 \eqdef \min\enscond{\norm{u-u_0}}{u\in \partial U_0}$.

Then,  the conclusions of Proposition \ref{prop:IFT} hold with $V \supset \Bb(v_0, \min\pa{r_0/M, R})$ and $\norm{J_g(v)} \leq M$.

\end{prop}
\begin{proof}
Define $V^* \eqdef \bigcup_{V\in\Vv} V$ where $\Vv$ is the collection of all open sets such that
\begin{itemize}
\item[(i)] $v_0\in V$
\item[(ii)]  $V$ is star-shaped with respect to $v_0$,
\item[(iii)]  $V\subset \Bb(v_0, R)$
\item[(iv)]  there exists a $\Cc^1$ function $g: V \to \RR^{m}$ such that $g(v_0) = u_0$ and for all $v\in V$, $f(g(v), v) = 0$.
\item[(v)]  $g(v) \subset U_0$.
\end{itemize}
Note that $\Vv$ is non-empty since we can apply the implicit function theorem to $f$ at $u_0$, $v_0$ to obtain a set $V$ and function $g$ which satisfies (i) to (v).
The collection $\Vv$ is stable by union and we can define $g^*$ on $V^*$ by
$$
g^*(v) = g(v), \qquad \text{if} \quad v\in V, \; V\in \Vv, \; g \text{ is the corresponding function}.
$$
We simply need to show that $V^* \supset \Bb(v_0, r_0/M)$.

Let $v\in V$ be of norm 1, and define
$$
r \eqdef \sup\enscond{r>0}{ v_0+ rv \in V^*}.
$$
Then, $r\in (0, R]$. Assume that $r<R$.
Let  $v_r \eqdef v_0+r v \in V^*$ and we can define $g^*(v_r) = \lim_{r'\to r} g^*(v_0+ r'v)$.  Since $ g^*(v_0+ r'v) \in U_0$ for all $r'<r$, we have $u\in \overline{U_0}$.  We claim that $u\in \partial U_0$ is on the boundary. Suppose $u \in U_0$. Then, by assumption, $ f(g^*(v_r), v_r) = 0$ and $\partial_u f(g^*(v_r), v_r)$ is invertible, we can therefore apply the IFT to construct neighbourhoods $U'$ around $g^*(v_r)$, $V'$ around $v_r$ to define a $\Cc^1$ function $g: V' \to \RR^m$ such that $g(v_r) = g^*(v_r)$ and for all $v\in V'$, $f(g(v), v) = 0$.  We can therefore extend the set $V^*$ to a set $V_r$ such that $V^* \subsetneq V_r$. This is a contradiction to the maximality of $V^*$. So, $g^*(v_r)\in \partial U_0$. Note that for all $t\in [0,1)$,  $v_0 + t rv \in V^* \subset \Bb(v_0, R)$, so $g(v_0 + t rv) \in U_0$. So, by assumption $\norm{J_g(v_0 + tr v)} \leq M$. Therefore,
$$
r_0 \leq \norm{g^*(v_r) - u_0} =\norm{ \int_0^1 J_g(v_0 + tr v) (r v) \mathrm{d}t } \leq M r
$$
Therefore, $r\geq \frac{r_0}{M}$.

\end{proof}

\begin{thm}\label{thm:stability}
Let $\epsilon>0$ and $X = \Phi \mestar + W$ where $W \in \RR^{T\times v}$ satisfies $\norm{W}_F \leq \epsilon$ and $\mestar = \sum_{s=1}^k C^*_s \delta(\theta-\theta^*_s)$. Suppose that $\Gamma\eqdef \Gamma_{\btheta^*, C^*}$ is full rank and $\eta_V$ is nondegenerate with respect to $\mestar$, then  there exists constants $\rho_1,\rho_2,\rho_3>0$ which depend only on $\eta_V$ and $\Gamma$ such that   for all  $\epsilon/\alpha \leq \rho_1$ and
$\alpha  \leq \rho_2 \min_s \norm{C_s^*}^2 $, 
  \eqref{eq:spglasso} recovers a unique solution of the form $ \sum_{s=1}^k  C_s \delta(\theta-\theta_s)$ with 
\begin{equation}\label{eq:error_bd}
\norm{ C^* - C}_F + \norm{ \btheta^* - \btheta}_F   \leq \rho_3 \pa{ \frac{ { \epsilon+\alpha}}{\min_s \norm{C_s^*}} }
\end{equation}  

\end{thm}

\begin{proof}

The goal is to define a $\Cc^1$ function $G: \RR^{T\times v}\times \RR_+ \to \RR^{N+kd}$ such that $(C, \btheta) \eqdef G(W, \alpha)$ corresponds to  a solution of \eqref{eq:spglasso} with data $X= D_{\btheta^*} (C^*)^\top + W$. We first use the implicit function theorem to define such a $G$, then show that it does indeed define a solution to \eqref{eq:spglasso}.

To this end,  let $N= \sum_{s}\abs{I_s}$ and define a function
$$
F:\RR_+^{N} \times \Tspace^k \times \RR^{T \times v}\times  \RR_+ \to \RR^{N + kd}
$$
so that given $C = \ens{C_s}_{s\in [k]}$ with $C_s \in \RR^{\abs{I_s}}$, $\btheta\in\Tspace^k$, $W\in \RR^{T\times v}$ and $\alpha \in \RR_+$,
 $$F(C,\btheta,W,\alpha) = \begin{bmatrix}
\pa{g_s(C,\btheta,W,\alpha)}_{s=1}^k\\
\pa{h_s(C,\btheta,W,\alpha)}_{s=1}^k
\end{bmatrix}$$
where $g_s(C,\btheta,W,\alpha) \in \RR^{\abs{I_s}}$ and $h_s (C,\btheta,W,\alpha)\in \RR^{d}$ are given by
$$
g_s (C,\btheta,W,\alpha)^\top = 
\pa{ \phi(\theta_s)^\top[D_\btheta \bar C^\top -D_{\btheta^*} (C^*)^\top - W ] }_{I_s}+ \alpha \pa{ \lambda_1 +  \lambda_2 \frac{C_s^\top}{\norm{C_s}}}
$$
and
$$
h_s (C,\btheta,W,\alpha) = J_{\phi}(\theta_s)^\top \pa{D_\btheta \bar C^\top - D_{\btheta^*} (C^*)^\top- W} \frac{\bar C_s}{\norm{C_s}_2}.
$$
Here, $\bar C\in \RR^{ v\times k}$ is the matrix with $s^{th}$ column satisfying  $(\bar C_s)_{I_s} = C_s$ and $(\bar C_s)_{I_s^c} = 0$.
Clearly, if $(C,\btheta)$ correspond to a solution of \eqref{eq:spglasso} with data $X= D_{\btheta^*} (C^*)^\top + W$, then $F(C,\btheta,W,\alpha) = 0$. Note also that $F(C^*, \btheta^*, 0,0) = 0$.

The partial derivatives of $g \eqdef (g_s)$ and $h \eqdef (h_s)$ are as follows: Define \begin{equation}\label{eq:Z}
Z \eqdef D_{\btheta}\bar C^\top - D_{\btheta^*} (C^*)^\top - W,
\end{equation}
then
\begin{align*}
\partial_c g &=  \proj_{\bold{I}} \pa{\Id_{v}\otimes  \Phi^\top_{\btheta} D_{\btheta}} \proj_{\bold{I}}^* + \alpha \lambda_2 \diag \pa{\frac{1}{\norm{C_s}}\Id_{\abs{I_s}} -\frac{ C_s C_s^\top}{\norm{C_s}^3}}_{s\in[k]}
\\
\partial_\theta g &=  \diag([ Z_{(:, I_s)}]^\top \JJ_\phi(\theta_s))_{s\in[k]} + {\pa{ C_j  \phi(\theta_s)^\top \JJ_\phi(\theta_j)}}_{s,j\in [k]}  
\\
\partial_\al g &=   \pa{\lambda_1 + \lambda_2 \frac{C_s}{\norm{C_s}}}_{s\in[k]} \\
\partial_w g &= \proj_{\bold{I}} (\Id_v \otimes \Phi^\top_{\btheta})
\end{align*}

Let  $\HH_\phi(\theta)^\top \in\RR^{d\times d\times T}$ so that is $(i,j,n)$ entries with $i,j\in [d]$ for the Hessian of $\phi_n(\theta_s)$. So, given a vector  $z\eqdef (z_n)_{n=1}^T$, $\HH_\phi(\theta)^\top  z= \sum_{n=1}^T z_n \nabla^2 \phi_j(\theta) \in \RR^{d\times d}$. Then,
\begin{align*}
\partial_c h &= \diag\pa{\JJ_\phi(\theta_s)^\top Z_{(:, I_s)}  \pa{\frac{1}{\norm{C_s}_2}\Id_{\abs{I_s}} - \frac{C_s C_s^\top}{\norm{C_s}^3}   }   }_{s\in[k]} + \pa{  [\frac{1}{\norm{C_s}_2}C_s^\top \otimes \JJ_\phi(\theta)^\top] [\Id_v \otimes D_{\btheta}]}_{s\in[k]}\\
\partial_{\btheta} h &= \diag\pa{\HH_\phi(\theta_s)^\top Z \frac{\bar C_s}{\norm{C_s}_2} }_s + \pa{  \frac{1}{\norm{C_j}_2}\JJ_\phi(\theta_j)^\top \JJ_\phi(\theta_s) \bar C_j^\top \bar C_s }_{j,s\in [k]}
\\
\partial_\alpha h &= \mathbf{0}_{kd}\\
\partial_w h &= -\pa{\frac{1}{\norm{C_s}_2}C_s^\top\otimes  \JJ_\phi(\theta_s)^\top }_{s\in [k]}
\end{align*}

We therefore have
$$
\partial_{(C,\btheta)}F =\pa{ \Gamma_{\btheta,C}^\top\Gamma_{\btheta,C} +Y } \begin{pmatrix}
\Id_{N} & \mathbf{0}_{N \times kd}\\
\mathbf{0}_{kd\times N } &\diag\pa{\norm{C_s}_2}_{s=1}^k \otimes \Id_{d}
\end{pmatrix}
$$
where 
$$
Y\eqdef  \begin{pmatrix}
\alpha \lambda_2 \diag \pa{\frac{1}{\norm{C_s}}\Id_{\abs{I_s}} -\frac{ C_s C_s^\top}{\norm{C_s}^3}} & \diag\pa{\frac{1}{\norm{C_s}_2} \JJ_\phi(\theta_s)^\top Z_{(:,I_s)}   }_{s\in[k]}^\top \\
 \diag\pa{\JJ_\phi(\theta_s)^\top Z_{(:,I_s)}  \frac{1}{\norm{C_s}_2} \pa{\Id_{\abs{I_s}} - \frac{C_s C_s^\top}{\norm{C_s}_2^2}  } }_{s\in[k]} &  \diag\pa{\HH_\phi(\theta_s)^\top Z \frac{C_s}{\norm{C_s}_2^2} }_s 
\end{pmatrix},
$$
and
$$
\partial_{(\alpha,W)} F =\begin{bmatrix}
 \begin{pmatrix}
 \pa{\lambda_1 + \lambda_2 \frac{C_s}{\norm{C_s}^2}}_s\\
 \mathbf{0}_{kd}
\end{pmatrix}, &
\Gamma_{\btheta,C}^\top
\end{bmatrix}
$$

\textbf{Application of implicit function theorem to obtain a candidate solution.}

To apply the quantitative implicit function theorem, we first bound $\norm{\Gamma_{\btheta,C}}$ and $\norm{Y}$: Define $$S = \ens{S_s}_{s=1}^k \qandq S^* = \ens{S^*_s}_{s=1}^k \qwhereq S_s \eqdef C_s/\norm{C_s}_2 \qandq  S_s^* \eqdef C_s^*/\norm{C_s^*}_2$$
\begin{itemize} 
\item[i)] \textbf{Bound on $ \norm{\partial_{\al,W} F}$:} 

Note that by Taylor's theorem, $ \norm{D_\btheta - D_{\btheta^*}} \leq  \norm{\btheta -\btheta^*}_F \max_\theta \norm{\JJ_\phi(\btheta)}$ and
\begin{align*}
 &\norm{S_s \otimes \JJ_\phi(\theta_s) -S_s^* \otimes \JJ_\phi(\theta_s^*)} \leq
  \norm{\pa{S_s - S_s^*} \otimes \JJ_\phi(\theta_s) } + \norm{ S_s^* \otimes (\JJ_\phi(\theta_s^*) -\JJ_\phi(\theta_s)) }\\
  &\leq   \norm{S_s -S_s^* }_2 \max_\theta \norm{\JJ_\phi(\theta)} + \norm{\theta_s -\theta_s^*} \norm{S_s^*}_2 \max_\theta \norm{\HH_\phi(\theta)}.
\end{align*}
Therefore
\begin{align*}
\norm{\Gamma_{\btheta,C} - \Gamma_{\btheta^*,C^*}}^2 &\leq  \norm{D_\btheta - D_{\btheta^*}}^2 + \sum_s \norm{S_s \otimes \JJ_\phi(\theta_s) - S_s^* \otimes \JJ_\phi(\theta_s^*)}^2\\
&\leq   \norm{\btheta -\btheta^*}_F^2 \max_\theta \norm{\JJ_\phi(\btheta)}^2 +   \norm{S - S^*}_F^2 \max_\theta \norm{\JJ_\phi(\theta)}^2 + \norm{\btheta -\btheta^*}^2  \max_\theta \norm{\HH_\phi(\theta)}^2\\
&\leq  A_1^2 \pa{\norm{S-S^*}_F^2 + \norm{\btheta  - \btheta^*}_F^2}
\end{align*}
where $$A_1^2 \eqdef    \max_\theta \norm{\HH_\phi(\theta)}^2 + \max_\theta \norm{\JJ_\phi(\btheta)}^2. $$

We can apply the bounds in i)  to deduce that
\begin{equation}
 \norm{\partial_{\al,w} F}  \lesssim \norm{\Gamma_{\btheta^*,C^*}} +  A_1 \pa{\norm{S-S^*}_F + \norm{\btheta  - \btheta^*}_F}
\end{equation}

\item[ii)]
Bounds for $\partial_{(C,\btheta)} F$  when $F(C,\btheta, W, \alpha) = 0$.
%\textbf{Bounds for $\partial_{(C,\btheta)} F$ :}
 We first bound $\norm{Y}$:
 \begin{align*}
\norm{Y} \lesssim \max_s \ens{\frac{1}{\norm{C_s}_2}}  \cdot \max_s\ens{\alpha \lambda_2, \norm{ \JJ_\phi(\theta_s)^\top Z  }, \norm{\HH_\phi(\theta_s)^\top Z S_s}}
\end{align*}
Let $U \eqdef \begin{pmatrix}
  \pa{\lambda_1 + \lambda_2 C_s/\norm{C_s}_2}\\
 \mathbf{0}_{kd}
\end{pmatrix}$. Then,
$$
 \Gamma_{\btheta}^\top Z + \alpha U = 0.
$$
By applying $\Gamma_\btheta (\Gamma_\btheta^\top \Gamma_\btheta)^{-1}$ to both sides, we obtain
\begin{align*}
0 &= Z -  \proj_{\Rr(\Gamma_\btheta)}^\perp Z +\alpha (\Gamma_\btheta^\top)^\dagger  U\\
&=Z +  \proj_{\Rr(\Gamma_\btheta)}^\perp \Gamma_{\btheta^*} \binom{C^*}{\mathbf{0}_{kd}} + \proj_{\Rr(\Gamma_\btheta)}^\perp  W + \alpha (\Gamma_\btheta^\top)^\dagger  U
\end{align*}
Therefore,
$$
\norm{Z} \leq \norm{ \proj_{\Rr(\Gamma_\btheta)}^\perp D_{\btheta^*} \binom{C^*}{\mathbf{0}_{kd}}} + \norm{W} + \alpha \norm{ (\Gamma_\btheta^\top)^\dagger  U}
$$
Note that
\begin{align*}
&\proj_{\Rr(\Gamma_{\btheta,C})}^\perp D_{\btheta^* } C^*= \proj_{\Rr(\Gamma_{\btheta,C})}^\perp \sum_s \phi\pa{\theta^*_s} (C^*_s)^\top  \\
&= 
\proj_{\Rr(\Gamma_{\btheta,C})}^\perp \sum_s \Big( \phi\pa{\theta_s} (C^*_s)^\top + (\theta_s -\theta^*_s)  \JJ_\phi\pa{\theta_s} (C^*_s)^\top   + \Oo(\norm{\btheta - \btheta^*}^2_F)\Big)\\
&= 
\proj_{\Rr(\Gamma_{\btheta,C})}^\perp \sum_s \Big( \phi\pa{\theta_s} (C^*_s)^\top + (\theta_s - \theta^*_s )  \JJ_\phi\pa{\theta_s} C_s^\top  \\
&\qquad\qquad +\Oo(\norm{C^* - C}_F \norm{\btheta - \btheta^*}_F) + \Oo(\norm{\btheta - \btheta^*}^2_F)\Big)\\
&= \Oo(\norm{\btheta - \btheta^*}_F^2 + \norm{C^* - C}_F \norm{\btheta - \btheta^*}_F) 
\end{align*}
Moreover, $(\Gamma_\btheta^\top)^\dagger U = Q^* + \Oo(\norm{\btheta - \btheta^*}_F) + \Oo(\norm{S - S^*}_F)$ where
$$
Q^* \eqdef (\Gamma_{\btheta^*}^\top)^\dagger   \begin{pmatrix}
{\lambda_1 + \lambda_2 C_s^*/\norm{C_s^*}_2}\\
 \mathbf{0}_{kd}
\end{pmatrix}.
$$
Therefore,
$$
\norm{Z} = \Oo\pa{ \norm{\btheta - \btheta^*}_F + \norm{C^* - C}_F  + \alpha + \norm{W} }
$$
and where $c = \min_s \norm{C_s}$.
$$
\norm{Y} = \Oo\pa{ c^{-1} \cdot \pa{ \norm{\btheta - \btheta^*}_F^2 + \norm{C^* - C}_F^2  + \alpha + \lambda_2 \alpha + \norm{W}  } }
$$
To show that $\partial_{(C,\btheta)} F$ is invertible, note that given square matrices $A,E$ where $A$ is invertible,  $(A+E)$  is also invertible with $\norm{(A+E)^{-1}} \leq 2\norm{A^{-1}}$ provided that $\norm{E}  \leq \frac{1}{2\norm{A^{-1}}}$. 
We therefore require that 
$$
 \norm{\btheta - \btheta^*}_F + \norm{C^* - C}_F  + \alpha(1 + \lambda_2 ) + \norm{W}   = \Oo\pa{c\cdot  \norm{(\Gamma_{\btheta^*}^\top \Gamma_{\btheta^*})^{-1}}^{-1}}
$$
\end{itemize}

We can therefore apply Proposition \ref{prop:IFT_quant} with $u_0 = (C^*, \btheta^*)$, $v_0 = (0, \mathbf{0}_{k\times d})$, $r_0 = r^*$, $R =  \Oo\pa{\frac{c}{1+\lambda_2}\cdot  \norm{(\Gamma_{\btheta^*}^\top \Gamma_{\btheta^*})^{-1}}^{-1}}$,
$$
U_0 = \Bb(C^*, r^*)  \times \Bb(\btheta^*, r^*) 
$$
where $r^* =  \Oo\pa{c\cdot  \norm{(\Gamma_{\btheta^*}^\top \Gamma_{\btheta^*})^{-1}}^{-1}}$ and $M= \Oo\pa{ \norm{(\Gamma_{\btheta^*}^\top \Gamma_{\btheta^*})^{-1}} /c}$  We can therefore define
$$
G : \Bb(v_0, R_0) \to  \RR^{N+kd}
, \qwhereq R_0 =\Oo( c^2 \cdot  \norm{(\Gamma_{\btheta^*}^\top \Gamma_{\btheta^*})^{-1}}^{-1}  )
$$
so that $G(\alpha, W) = (C,\btheta)$ if and only if $F(C,\btheta,\alpha,W) = 0$, and
$$
\norm{C-C^*}_F+ \norm{\btheta - \btheta^*}_F \lesssim (\alpha+\norm{W}_F)/c.
$$

\textbf{Verifying the candidate solution.}
Finally, it remains to check  that $G(\alpha, W) = (C,\btheta)$ does indeed correspond to a solution: it suffices to check that $$Q \eqdef \frac{-1}{\alpha}Z = \frac{-1}{\alpha} (D_{\btheta} \bar C - D_{\btheta^*} C^* - W)$$ satisfies the primal dual relationships (see Lemma \ref{lem:pd}). In particular, we need to check that $\eta \eqdef \Phi^* P$ satisfies $ \sup_{\theta\in\Tspace} \norm{ \frac{1}{\lambda_2}(\eta(\theta) - \lambda_1)_+}_2 \leq 1$.
Note that $F(C,\btheta,\alpha,W) = 0$ can be rewritten as
$$
\Gamma_{\btheta,C}^\top Z  = -  \begin{pmatrix}
 \alpha(\lambda_1 + \lambda_2 \frac{C_s}{\norm{C_s}})_{s\in[k]}\\
 \mathbf{0}_{kd}
\end{pmatrix} .
$$
 By applying $\Gamma_{\btheta,C} (\Gamma_{\btheta,C}^\top\Gamma_{\btheta,C})^{-1}$ to this equation and recalling that $\proj_{\Rr(\Gamma_{\btheta,C})} \eqdef \Gamma_{\btheta,C} (\Gamma_{\btheta,C}^\top\Gamma_{\btheta,C})^{-1} \Gamma_{\btheta,C}^\top$ is the orthogonal projection onto the range of $\Gamma_{\btheta,C}$, we obtain
\begin{align*}
-\frac{1}{\al} Z =  (\Gamma_{\btheta,C}^\top)^\dagger u_0
-\frac{1}{\alpha} \proj_{\Rr(\Gamma_{\btheta,C})}^\perp  (D_{\btheta^*} C^* + W)
\end{align*}
It therefore follows that $Q = Q_V  -\frac{1}{\alpha} \proj_{\Rr(\Gamma_{\btheta,C})}^\perp  (D_{\btheta^*} C^* + W)$.  Let $\eta \eqdef \Phi^* P$. We need to show that $g(\theta) \eqdef \norm{\frac{1}{\lambda_2}[\eta(\theta) - \lambda_1]_+ }^2_2$ satisfies
\begin{itemize}
\item[i)] $g(\theta) <1$ for all $\theta \not\in \btheta$
\item[ii)]  $g''(\theta_s) \neq 0$ for all $s\in [k]$. 
\end{itemize}
Note that since $\abs{\eta(\theta)  - \eta_V(\theta)} \leq \max_\theta \norm{\phi(\theta)}_2 \norm{Q - Q_V}_F =  \norm{Q - Q_V}_F$
and
$$
\abs{\eta(\theta)  - \eta_V(\theta)} \leq \max_\theta \norm{\HH_\phi(\theta)} \norm{Q - Q_V}_F,
$$
 provided that $  \norm{Q - Q_V}_F$ is sufficiently small, we have $\eta_i(\theta)>\lambda_1$  whenever  $(\eta_V)_i(\theta)>\lambda_1$ and $g$ satisfies i) and ii) since $\eta_V$ is nondegenerate.

%Note that for scalars $a,b$, $$\abs{\max(a,0)^2 - \max(b,0)^2}  \leq ( \max(a,0) +  \max(b,0)) \cdot \abs{a-b} \leq \abs{a-b}^2 +2\max(b,0)\cdot \abs{a-b}$$
%so,
%\begin{align*}
%\abs{g(\theta) - g_V(\theta) } &\leq
%\frac{1}{\lambda_2} \sum_{i=1}^v \abs{[\eta_i (\theta) - \lambda_1]_+^2 - [(\eta_V)_i (\theta) - \lambda_1]_+ ^2  }\\
%&\leq \frac{1}{\lambda_2} \sum_{i=1}^v \abs{\eta_i (\theta) -(\eta_V)_i (\theta) }^2 + 2  [(\eta_V)_i (\theta) - \lambda_1]_+ \abs{\eta_i (\theta) -(\eta_V)_i (\theta) }\\
%&\leq \frac{1}{\lambda_2} \pa{ \norm{\eta(\theta) - \eta_V(\theta)}^2_2 + 2 \sqrt{g_V(\theta)} \norm{\eta(\theta) - \eta_V(\theta)}_2}\\
%&\leq \frac{1}{\lambda_2} \pa{  \norm{\phi(\theta)}_2^2 \norm{P-Q_V}^2_F + 2 \sqrt{g_V(\theta)}  \norm{\phi(\theta)}_2\norm{P-Q_V}_F}\\
%&=\frac{1}{\lambda_2} \pa{ \norm{P-Q_V}^2_F + 2 \sqrt{g_V(\theta)}  \norm{P-Q_V}_F}
%\end{align*}
%Similarly,
%$$
%\norm{\nabla^2 g(\theta) - \nabla^2 g_V(\theta)} \leq \frac{1}{\lambda_2} \pa{  \norm{\nabla^2 \phi(\theta)}_2^2 \norm{P-Q_V}^2_F + 2 \sqrt{g_V(\theta)}  \norm{\nabla^2 \phi(\theta)}_2\norm{P-Q_V}_F}
%$$

% and $\max_\theta \norm{\partial^{(j)} \eta(\theta) -\partial^{(j)} \eta_V(\theta)} \lesssim \norm{Q_V - Q}_F$ where the hidden constant depends only on $\max_{\theta}\norm{\partial^{(j)} \phi(\theta)}$,  
 
 It is enough to show that $\norm{Q_V - Q}_F \leq \rho$ for a sufficiently small constant $\rho$ (which depends only on $\eta_V$, and in particular, $\min_{i\in I_s} (\eta_V)_i(\theta^*_s) - \lambda_1$, $g_V''(\theta^*_s)$ and $1-g_V(\theta)$ for $\theta \not\in  \cup_s \Bb(\theta^*_s,r)$ where $r$ is such that $\min_{\theta\in \Bb(\theta_s,r)}\abs{g_V''(\theta)}\geq \frac12 \abs{g_V''(\theta_s)}$ ). Note that
\begin{align*}
&\proj_{\Rr(\Gamma_{\btheta,C})}^\perp D_{\btheta^* } C^*= \proj_{\Rr(\Gamma_{\btheta,C})}^\perp \sum_s \phi\pa{\theta^*_s} (C^*_s)^\top  \\
&= 
\proj_{\Rr(\Gamma_{\btheta,C})}^\perp \sum_s \Big( \phi\pa{\theta_s} (C^*_s)^\top + (\theta_s -( \theta_0)_s)  \JJ_\phi\pa{\theta_s} (C^*_s)^\top  \\
&\qquad\qquad + \Oo(\norm{\btheta - \btheta^*}^2_F)\Big)\\
&= 
\proj_{\Rr(\Gamma_{\btheta,C})}^\perp \sum_s \Big( \phi\pa{\theta_s} (C^*_s)^\top + (\theta_s -( \theta_0)_s)  \JJ_\phi\pa{\theta_s} C_s^\top  \\
&\qquad\qquad +\Oo(\norm{C^* - C}_F \norm{\btheta - \btheta^*}_F) + \Oo(\norm{\btheta - \btheta^*}^2_F)\Big)\\
&= \Oo(\norm{\btheta - \btheta^*}_F^2 + \norm{C^* - C}_F \norm{\btheta - \btheta^*}_F) = \Oo(\alpha^2/c^2)
\end{align*}
So, $Q = Q_V + \Oo( \norm{W}_F/\alpha + \alpha/c^2)$, and so, $C,\btheta$ define a solution provided that $\norm{W}_F/\alpha + \alpha/c^2 = \Oo(1)$.

\end{proof}
