# Supplementary material for: An off-the-grid approach to multi-compartment magnetic resonance fingerprinting
Source: arXiv:2011.11193 source file (2020-11-23)
Supplement: Supplementary file 2 [file supp.tex]

%======
\section{Results and discussions}
\subsection{Network embedding of Bloch responses}

%=====brainweb GTmaps=====
\begin{figure}[t]
	\centering
	\scalebox{1}{
	\begin{minipage}{\linewidth}
		\centering		
\includegraphics[width=.5\linewidth]{../figs_gen/Table_paper/trainingcurve_1000.pdf}
\end{minipage}}
\caption{{Training and validation MSE losses during training the neural network model to approximate Bloch responses. 
}\label{fig:trainingcurve} }
\end{figure}

%===================

\subsection{Numerical box phantom experiment}

\begin{figure*}[t]
	\centering	
	\scalebox{1}{
	\begin{minipage}{\linewidth}
		\centering	
%\begin{turn}{90} mixtures scatter plot \end{turn}
\includegraphics[width=.19\linewidth]{../figs_gen/synth/figs_expe2/expe2_diri_distr1.pdf}
\includegraphics[width=.19\linewidth]{../figs_gen/synth/figs_expe2/expe2_diri_distr2.pdf}
\includegraphics[width=.19\linewidth]{../figs_gen/synth/figs_expe2/expe2_diri_distr3.pdf}
\includegraphics[width=.19\linewidth]{../figs_gen/synth/figs_expe2/expe2_diri_distr4.pdf}
\includegraphics[width=.19\linewidth]{../figs_gen/synth/figs_expe2/expe2_diri_distr5.pdf}
\\
$a=0.1$ \hspace{2.5cm}$a=0.5$ \hspace{2.5cm}$a=1$ \hspace{2.5cm}$a=2$ \hspace{2.5cm}$a=4$ 
\\
\vspace{.2cm}
(a) Scatter plot of the pixels' mixture weights across the three compartments. \vspace{.3cm}
\\
\begin{turn}{90} \,1st compartment \end{turn}
\includegraphics[width=.15\linewidth]{../figs_gen/synth/figs_expe2/expe2_diri_maps11c.pdf}\hspace{.3cm}
\includegraphics[width=.15\linewidth]{../figs_gen/synth/figs_expe2/expe2_diri_maps21c.pdf}\hspace{.3cm}
\includegraphics[width=.15\linewidth]{../figs_gen/synth/figs_expe2/expe2_diri_maps31c.pdf}\hspace{.3cm}
\includegraphics[width=.15\linewidth]{../figs_gen/synth/figs_expe2/expe2_diri_maps41c.pdf}\hspace{.3cm}
\includegraphics[width=.15\linewidth]{../figs_gen/synth/figs_expe2/expe2_diri_maps51c.pdf}
\begin{turn}{90} \includegraphics[width=.13\linewidth]{../figs_gen/brainweb/figs_expe3_cut/mixmaps_new/colorbarMaps_c.pdf}\end{turn}
\\
%(b) Mixture maps of the first compartment (T1/T2 $=784/77$). \vspace{.2cm}
%\\
\begin{turn}{90} 2nd compartment \end{turn}
\includegraphics[width=.15\linewidth]{../figs_gen/synth/figs_expe2/expe2_diri_maps12c.pdf}\hspace{.3cm}
\includegraphics[width=.15\linewidth]{../figs_gen/synth/figs_expe2/expe2_diri_maps22c.pdf}\hspace{.3cm}
\includegraphics[width=.15\linewidth]{../figs_gen/synth/figs_expe2/expe2_diri_maps32c.pdf}\hspace{.3cm}
\includegraphics[width=.15\linewidth]{../figs_gen/synth/figs_expe2/expe2_diri_maps42c.pdf}\hspace{.3cm}
\includegraphics[width=.15\linewidth]{../figs_gen/synth/figs_expe2/expe2_diri_maps52c.pdf}
\begin{turn}{90} \includegraphics[width=.13\linewidth]{../figs_gen/brainweb/figs_expe3_cut/mixmaps_new/colorbarMaps_c.pdf}\end{turn}
\\
%(c) Mixture maps of the second compartment (T1/T2 $=1216/96$). \vspace{.2cm}
%\\
\begin{turn}{90}  3rd compartment \end{turn}
\includegraphics[width=.15\linewidth]{../figs_gen/synth/figs_expe2/expe2_diri_maps13c.pdf}\hspace{.3cm}
\includegraphics[width=.15\linewidth]{../figs_gen/synth/figs_expe2/expe2_diri_maps23c.pdf}\hspace{.3cm}
\includegraphics[width=.15\linewidth]{../figs_gen/synth/figs_expe2/expe2_diri_maps33c.pdf}\hspace{.3cm}
\includegraphics[width=.15\linewidth]{../figs_gen/synth/figs_expe2/expe2_diri_maps43c.pdf}\hspace{.3cm}
\includegraphics[width=.15\linewidth]{../figs_gen/synth/figs_expe2/expe2_diri_maps53c.pdf}
\begin{turn}{90} \includegraphics[width=.13\linewidth]{../figs_gen/brainweb/figs_expe3_cut/mixmaps_new/colorbarMaps_c.pdf}\end{turn}
\\
$a=0.1$ \hspace{2cm}$a=0.5$ \hspace{2cm}$a=1$ \hspace{2cm}$a=2$ \hspace{2cm}$a=4$ 
\\
\vspace{.2cm}
(b) Mixture maps of the three compartments. 
\caption{Exemplar mixture weights used for simulating the $20\times20$ pixel box phantom from three compartments: (a) distribution of the pixels' mixture weights, (b) per-compartment mixture maps. Mixture weights are drawn at random from dirichlet distributions with different parameters $a$: large $a$ values result in highly mixed pixels that are more difficult to separate, whereas small $a$ values lead to sparser mixture maps that are easier to demix. 
}\label{fig:diri_maps} 
\end{minipage}}
\end{figure*}

\subsection{Numerical Brain phantom experiment}

\begin{figure*}[t]
	\centering
	\scalebox{.95}{
	\begin{minipage}{\linewidth}
		\centering	
		WM \hspace{2cm}$\Delta$ WM	\hspace{2cm} GM \hspace{2cm}$\Delta$ GM \hspace{2cm} CSF\hspace{2cm}$\Delta$ CSF\vspace{.1cm}\\
\begin{turn}{90} \quad\qquad Full \end{turn}
\includegraphics[width=.15\linewidth]{../figs_gen/brainweb/figs_expe3_cut/mixmaps_new/expe3_cut_im_3351c.pdf}\hspace{-.1cm}
\includegraphics[width=.15\linewidth]{../figs_gen/brainweb/figs_expe3_cut/mixmaps_new/expe3_cut_im_diff_3351.pdf}\hspace{.1cm}
\includegraphics[width=.15\linewidth]{../figs_gen/brainweb/figs_expe3_cut/mixmaps_new/expe3_cut_im_3352c.pdf}\hspace{-.1cm}
\includegraphics[width=.15\linewidth]{../figs_gen/brainweb/figs_expe3_cut/mixmaps_new/expe3_cut_im_diff_3352.pdf}\hspace{.1cm}
\includegraphics[width=.15\linewidth]{../figs_gen/brainweb/figs_expe3_cut/mixmaps_new/expe3_cut_im_3353c.pdf}\hspace{-.1cm}
\includegraphics[width=.15\linewidth]{../figs_gen/brainweb/figs_expe3_cut/mixmaps_new/expe3_cut_im_diff_3353.pdf}
\\
\begin{turn}{90} \quad\qquad LRTV \end{turn}
\includegraphics[width=.15\linewidth]{../figs_gen/brainweb/figs_expe3_cut/mixmaps_new/expe3_cut_im_3151c.pdf}\hspace{-.1cm}
\includegraphics[width=.15\linewidth]{../figs_gen/brainweb/figs_expe3_cut/mixmaps_new/expe3_cut_im_diff_3151.pdf}\hspace{.1cm}
\includegraphics[width=.15\linewidth]{../figs_gen/brainweb/figs_expe3_cut/mixmaps_new/expe3_cut_im_3152c.pdf}\hspace{-.1cm}
\includegraphics[width=.15\linewidth]{../figs_gen/brainweb/figs_expe3_cut/mixmaps_new/expe3_cut_im_diff_3152.pdf}\hspace{.1cm}
\includegraphics[width=.15\linewidth]{../figs_gen/brainweb/figs_expe3_cut/mixmaps_new/expe3_cut_im_3153c.pdf}\hspace{-.1cm}
\includegraphics[width=.15\linewidth]{../figs_gen/brainweb/figs_expe3_cut/mixmaps_new/expe3_cut_im_diff_3153.pdf}
\\
\begin{turn}{90} \qquad SVD-MRF \end{turn}
\includegraphics[width=.15\linewidth]{../figs_gen/brainweb/figs_expe3_cut/mixmaps_new/expe3_cut_im_3251c.pdf}\hspace{-.1cm}
\includegraphics[width=.15\linewidth]{../figs_gen/brainweb/figs_expe3_cut/mixmaps_new/expe3_cut_im_diff_3251.pdf}\hspace{.1cm}
\includegraphics[width=.15\linewidth]{../figs_gen/brainweb/figs_expe3_cut/mixmaps_new/expe3_cut_im_3252c.pdf}\hspace{-.1cm}
\includegraphics[width=.15\linewidth]{../figs_gen/brainweb/figs_expe3_cut/mixmaps_new/expe3_cut_im_diff_3252.pdf}\hspace{.1cm}
\includegraphics[width=.15\linewidth]{../figs_gen/brainweb/figs_expe3_cut/mixmaps_new/expe3_cut_im_3253c.pdf}\hspace{-.1cm}
\includegraphics[width=.15\linewidth]{../figs_gen/brainweb/figs_expe3_cut/mixmaps_new/expe3_cut_im_diff_3253.pdf}
\\
(a) Sequence length $T=500$ \vspace{.2cm}
\\
\begin{turn}{90} \quad\qquad Full \end{turn}
\includegraphics[width=.15\linewidth]{../figs_gen/brainweb/figs_expe3_cut/mixmaps_new/expe3_cut_im_4351c.pdf}\hspace{-.1cm}
\includegraphics[width=.15\linewidth]{../figs_gen/brainweb/figs_expe3_cut/mixmaps_new/expe3_cut_im_diff_4351.pdf}\hspace{.1cm}
\includegraphics[width=.15\linewidth]{../figs_gen/brainweb/figs_expe3_cut/mixmaps_new/expe3_cut_im_4352c.pdf}\hspace{-.1cm}
\includegraphics[width=.15\linewidth]{../figs_gen/brainweb/figs_expe3_cut/mixmaps_new/expe3_cut_im_diff_4352.pdf}\hspace{.1cm}
\includegraphics[width=.15\linewidth]{../figs_gen/brainweb/figs_expe3_cut/mixmaps_new/expe3_cut_im_4353c.pdf}\hspace{-.1cm}
\includegraphics[width=.15\linewidth]{../figs_gen/brainweb/figs_expe3_cut/mixmaps_new/expe3_cut_im_diff_4353.pdf}
\\
\begin{turn}{90} \quad\qquad LRTV \end{turn}
\includegraphics[width=.15\linewidth]{../figs_gen/brainweb/figs_expe3_cut/mixmaps_new/expe3_cut_im_4151c.pdf}\hspace{-.1cm}
\includegraphics[width=.15\linewidth]{../figs_gen/brainweb/figs_expe3_cut/mixmaps_new/expe3_cut_im_diff_4151.pdf}\hspace{.1cm}
\includegraphics[width=.15\linewidth]{../figs_gen/brainweb/figs_expe3_cut/mixmaps_new/expe3_cut_im_4152c.pdf}\hspace{-.1cm}
\includegraphics[width=.15\linewidth]{../figs_gen/brainweb/figs_expe3_cut/mixmaps_new/expe3_cut_im_diff_4152.pdf}\hspace{.1cm}
\includegraphics[width=.15\linewidth]{../figs_gen/brainweb/figs_expe3_cut/mixmaps_new/expe3_cut_im_4153c.pdf}\hspace{-.1cm}
\includegraphics[width=.15\linewidth]{../figs_gen/brainweb/figs_expe3_cut/mixmaps_new/expe3_cut_im_diff_4153.pdf}
\\
\begin{turn}{90} \qquad SVD-MRF \end{turn}
\includegraphics[width=.15\linewidth]{../figs_gen/brainweb/figs_expe3_cut/mixmaps_new/expe3_cut_im_4251c.pdf}\hspace{-.1cm}
\includegraphics[width=.15\linewidth]{../figs_gen/brainweb/figs_expe3_cut/mixmaps_new/expe3_cut_im_diff_4251.pdf}\hspace{.1cm}
\includegraphics[width=.15\linewidth]{../figs_gen/brainweb/figs_expe3_cut/mixmaps_new/expe3_cut_im_4252c.pdf}\hspace{-.1cm}
\includegraphics[width=.15\linewidth]{../figs_gen/brainweb/figs_expe3_cut/mixmaps_new/expe3_cut_im_diff_4252.pdf}\hspace{.1cm}
\includegraphics[width=.15\linewidth]{../figs_gen/brainweb/figs_expe3_cut/mixmaps_new/expe3_cut_im_4253c.pdf}\hspace{-.1cm}
\includegraphics[width=.15\linewidth]{../figs_gen/brainweb/figs_expe3_cut/mixmaps_new/expe3_cut_im_diff_4253.pdf}
\\
\hspace{.2cm}
\includegraphics[width=.14\linewidth]{../figs_gen/brainweb/figs_expe3_cut/mixmaps_new/colorbarMaps_c.pdf}\hspace{0.1cm}
\includegraphics[width=.14\linewidth]{../figs_gen/brainweb/figs_expe3_cut/mixmaps_new/colorbardiffMaps.pdf}\hspace{0.1cm}
\includegraphics[width=.14\linewidth]{../figs_gen/brainweb/figs_expe3_cut/mixmaps_new/colorbarMaps_c.pdf}\hspace{0.1cm}
\includegraphics[width=.14\linewidth]{../figs_gen/brainweb/figs_expe3_cut/mixmaps_new/colorbardiffMaps.pdf}\hspace{0.1cm}
\includegraphics[width=.14\linewidth]{../figs_gen/brainweb/figs_expe3_cut/mixmaps_new/colorbarMaps_c.pdf}\hspace{0.1cm}
\includegraphics[width=.14\linewidth]{../figs_gen/brainweb/figs_expe3_cut/mixmaps_new/colorbardiffMaps.pdf}
\\
(b) Sequence length $T=250$
\end{minipage}}
\caption{{The estimated T1/T2 values, (normalised) mixture maps and their differences ($\Delta$) with the ground truth for the WM, GM and CSF compartments of the simulated brain phantom using \MCMRF algorithm. For various sequence lengths $T$, the TSMIs were either un-compressed (Full) or subsampled using compressed sensing (i.e. the same acquisition protocol used in  \emph{in-vivo} experiments) and reconstructed with the LRTV and SVD-MRF schemes before mixture separation. \todo{why SVDMRF k=500 is worst than 250! find another example}
}\label{fig:brainweb_SGBlasso} }
\end{figure*}

\subsection{Truncated sequence}

\begin{figure*}[ht!]
	\centering
	\scalebox{1}{
	\begin{minipage}{\linewidth}
		\centering		
\begin{turn}{90} \qquad $T = 750$\end{turn}
\includegraphics[width=.155\linewidth]{../figs_gen/vivo/figs_expe3_cut/im_1511c.pdf}\vspace{-.1cm}
\includegraphics[width=.155\linewidth]{../figs_gen/vivo/figs_expe3_cut/im_1512c.pdf}\vspace{-.1cm}
\includegraphics[width=.155\linewidth]{../figs_gen/vivo/figs_expe3_cut/im_1513c.pdf}\vspace{.2cm}
\includegraphics[width=.155\linewidth]{../figs_gen/vivo/figs_expe3_cut/im_2511c.pdf}\vspace{-.1cm}
\includegraphics[width=.155\linewidth]{../figs_gen/vivo/figs_expe3_cut/im_2512c.pdf}\vspace{-.1cm}
\includegraphics[width=.155\linewidth]{../figs_gen/vivo/figs_expe3_cut/im_2513c.pdf}\vspace{.2cm}
\\
\begin{turn}{90} \qquad $T=500$\end{turn}
\includegraphics[width=.155\linewidth]{../figs_gen/vivo/figs_expe3_cut/im_1521c.pdf}\vspace{-.1cm}
\includegraphics[width=.155\linewidth]{../figs_gen/vivo/figs_expe3_cut/im_1522c.pdf}\vspace{-.1cm}
\includegraphics[width=.155\linewidth]{../figs_gen/vivo/figs_expe3_cut/im_1523c.pdf}\vspace{.2cm}
\includegraphics[width=.155\linewidth]{../figs_gen/vivo/figs_expe3_cut/im_2521c.pdf}\vspace{-.1cm}
\includegraphics[width=.155\linewidth]{../figs_gen/vivo/figs_expe3_cut/im_2522c.pdf}\vspace{-.1cm}
\includegraphics[width=.155\linewidth]{../figs_gen/vivo/figs_expe3_cut/im_2523c.pdf}\vspace{.2cm}
\\
\begin{turn}{90} \qquad $T=250$\end{turn}
\includegraphics[width=.155\linewidth]{../figs_gen/vivo/figs_expe3_cut/im_1531c.pdf}\vspace{-.1cm}
\includegraphics[width=.155\linewidth]{../figs_gen/vivo/figs_expe3_cut/im_1532c.pdf}\vspace{-.1cm}
\includegraphics[width=.155\linewidth]{../figs_gen/vivo/figs_expe3_cut/im_1533c.pdf}\vspace{.2cm}
\includegraphics[width=.155\linewidth]{../figs_gen/vivo/figs_expe3_cut/im_2531c.pdf}\vspace{-.1cm}
\includegraphics[width=.155\linewidth]{../figs_gen/vivo/figs_expe3_cut/im_2532c.pdf}\vspace{-.1cm}
\includegraphics[width=.155\linewidth]{../figs_gen/vivo/figs_expe3_cut/im_2533c.pdf}\vspace{.2cm}
\\
(a) methods used LRTV reconstruction\hspace{3cm} (b) methods used SVD-MRF reconstruction
\caption{{Estimated mixture maps and their T1/T2s for the WM, GM and CSF in-vivo brain compartments using \MCMRF at truncated sequence lengths $T$. Methods used (a) LRTV or (b) SVD-MRF reconstructions before mixture separation. 
}\label{fig:vivo_cut_blasso} }
\end{minipage}}
\end{figure*}
