# Supplementary material for: An off-the-grid approach to multi-compartment magnetic resonance fingerprinting
Source: arXiv:2011.11193 source file (2020-11-23)
Supplement: Supplementary file 3 [file supp_theory_old.tex]

% !TEX root = ../offgridQMRI.tex

\newcommand{\JJ}{\mathbb{J}}
\newcommand{\HH}{\mathbb{H}}

\section{Support stability}

\paragraph{Notations}
 For $\phi:\RR^d \to \RR^T$, let $\JJ_\phi(\theta) \in \RR^{T\times d}$ denote the Jacobian of $\phi$ at $\theta$.   Given a matrix $Q\in \RR^{n\times m}$, let $\vc_{n,m}(p)\in\RR^{nm}$ be its vectorized version with columns stacked vertically, let $\rc_{n,m}$ be the inverse operation, so that $\rc_{n,m}(\vc_{n,m}(p)) = p$. Finally, we define the soft-thresholding operator by $S_\beta:\RR^v \to \RR^v$ is defined by  $$S_\beta(\xi)_i = \begin{cases} \xi_i -\beta &\xi_i >\beta,
\\ \xi_i +\beta &\xi_i<-\beta,
 \\0  & \abs{\xi_i}\leq \beta.
\end{cases}.$$
Given a matrix or a tensor, we write  $\norm{\cdot}$ without subscript to denote the operator norm with respect to the vector norm $\norm{\cdot}_2$. Given an index set $I$ and a vector $V$, we denote by $\proj_I(V)$ the restriction of $V$ to the index set $I$. Given a point $x\in \RR^n$ and $r>0$, we denote by $\Bb(x,r) \eqdef \enscond{z}{\norm{x-z}<r}$ the open ball of radius $r$ around $x$.

\subsection{The precertificate as a least squares solution}\label{supp:precertificate_lsq}
We detail here how to write the solution of $Q_V$ as the solution of a linear system. Observe that the constraints $\proj_{I_s}f(\theta_s) = \frac{\proj_{I_s}C_s}{\norm{C_s}_2}$ for all $s\in [k]$ can be written as
\begin{align*}
\proj_{\bold{I}} \vc_{k,v} \pa{ \Phi^\top_{\btheta} Q}= \proj_{\bold{I}} [\Id_v \otimes D_{\btheta}^\top]\vc_{T,v}(P) = u_0
\end{align*}
where $u_0 = \pa{(1-\beta) +\beta  \sqrt{v}\proj_{I_s}  C_s/\norm{C_s}_2}_{s=1}^k \in \RR^{\sum_s \abs{I_s}}$ and 
$\proj_{\bold{I}}: \RR^{kv} \to \RR^{\sum_s \abs{I_s}}$ is the  subsampling operator given  by which selects the nonzero entries of $\ens{I_s}_{s\in[k]}$, so that given a matrix $z \in \RR^{k\times v}$ with $s^{th}$ row $z_s \in \RR^{v}$ for $s\in [k]$, $\proj_{\bold{I}} \vc(z) = \pa{(z_s)_{I_s}}_{s\in [k]}$.

The constraints $\partial_\theta \norm{f(\theta_s)}_2^2 = 0$  for all $s\in [k]$ can be written as
\begin{align*}
\mathbf{0}_d &= \beta \sqrt{v} \sum_{i\in I_s}  f_i(\theta_s) \nabla f_i(\theta_s)  = \frac{1}{\norm{C_s}_2} \sum_{i=1}^v (C_s)_i \nabla [\Phi^* Q](\theta_s) \\
&= \JJ_\phi(\theta_s)^\top Q \frac{C_s}{\norm{C_s}_2} =\frac{1}{\norm{C_s}_2}[ C_s^\top\otimes \JJ_\phi(\theta_s)^\top]\vc_{T,v}(P)
\end{align*}

We can therefore define the $Tv\times (\sum_{s=1}^k \abs{I_s}+kd)$ matrix \begin{equation}\label{eq:Gamma}
\Gamma = \left[(\Id_v\otimes D_\btheta ) \proj_{\bold{I}}^* ,\frac{ C_1}{\norm{C_1}_2} \otimes \JJ_\phi(\theta_1), \cdots, ,\frac{ C_k}{\norm{C_k}_2} \otimes \JJ_\phi(\theta_k) \right]
 \end{equation}
 and write
 $Q_V = \rc_{T,v} \pa{(\Gamma^*)^\dagger \begin{pmatrix}
u_0\\
\mathbf{0}_{kd}
\end{pmatrix}}$. Note that $\Gamma$ depends on $\btheta$ and $C$. To make this dependence clear, we will sometimes write $\Gamma_{\btheta,C}$ in place of $\Gamma$.

\subsection{The dual of sparse group Blasso}

The proof of Theorem \ref{thm:stability} is via analysis of the dual problem to \eqref{eq:spglasso}.  The proof follows closely the proof of support stability from \cite{duval2015exact}, however, we present the details here since the case of vector-valued measured with the sparse group norm has not be covered in the literature. 
We describe the some primal dual relationships in this section.

To simplify notation, throughout this section and the next, we let  $\lambda_1 \eqdef \beta$ and $\lambda_2 \eqdef \sqrt{v}(1-\beta)$.



\paragraph{Duality for sparse group lasso}
Before describing the dual problem, we first mention a duality, described in \cite{burdakov2001new}, between the vector norm (for $x\in\RR^n$ and $\epsilon>0$), $J(x) \eqdef  \epsilon \norm{x}_1 + (1-\epsilon)\norm{x}_2$, and the so-called $\epsilon$-norm, which is defined for $\xi\in\RR^n$ as  $\nu = \norm{\xi}_\epsilon$  is the unique $\nu>0$ such that
$$
\sum_i (\abs{\xi_i} - (1-\epsilon)\nu)_+^2 - (\epsilon \nu)^2 = 0.
$$
It is shown in \cite[Appendix E, Lemmas 1 and 2]{ndiaye2016gap} (see also \cite{burdakov2001new}) that \footnote{which of course can be written as: for all $\lambda_1,\lambda_2>0$, \begin{equation*}
\begin{split}
&\enscond{x+y}{\norm{x}_2 \leq \lambda_1 \nu, \norm{y}_\infty \leq\lambda_2 \nu} = \enscond{\xi}{  \norm{S_{\lambda_2}(\xi)}^2_2 \leq  (\lambda_1 \nu)^2 }
\end{split}
\end{equation*}}
\begin{equation}\label{eq:epsnorm1}
\begin{split}
&\enscond{x+y}{x,y\in\RR^d, \norm{x}_2 \leq \epsilon \nu, \norm{y}_\infty \leq (1-\epsilon) \nu} \\
&= \enscond{\xi\in \RR^d}{\norm{\xi}_\epsilon \leq \nu}
\end{split}
\end{equation}
and hence, the dual norm of $J$ is the $\epsilon$-norm. Moreover, we have the \emph{unique} $\epsilon$-decomposition
$$
\xi = S_\epsilon(\xi) + (\xi - S_\epsilon(\xi) )
$$
with $\norm{S_\epsilon(\xi)}_2 = (1-\epsilon) \norm{\xi}_\epsilon$ and $\norm{\xi - S_\epsilon(\xi) }_\infty = \epsilon\norm{\xi}_\epsilon$,
where we recall that $S_\epsilon$ is the soft-thresholding operator.

 
 \paragraph{The dual of sparse group Blasso}
 \begin{lem}\label{lem:pd}
 The dual problem to \eqref{eq:spglasso} is
 \eql{\label{eq:spglassodual}
\sup_{Q \in K} \dotp{X}{Q}_F - \alpha \norm{Q}_F^2 \tag{$\Dd_\al(X)$}
}
where $\Kk \subseteq \RR^{T\times v}$ is defined as
$$
\Kk  \eqdef 
\enscond{Q}{\eta \eqdef \Phi^* Q, \; \sum_{i=1}^v ({\eta_i(\theta)} - \lambda_1 )_+^2 \leq \lambda_2^2}
 $$
 The primal and dual problems are related by $\meas$ solves \eqref{eq:spglasso} if and only if $Q= \frac{X-\Phi \meas }{\alpha}$ solves \eqref{eq:spglassodual}.  Moreover, $\Phi^* Q \in \partial \norm{\meas}_\beta$.
 \end{lem}
\begin{proof}
By considering the dual norms of $\abs{\meas}_1$ and $\abs{\meas}_2$, it holds
\begin{equation}\label{eq:eps_decomp}
\begin{split}
&\norm{\meas}_\beta =  \sup_{\sup_\theta\norm{f(\theta)}_\infty \leq \beta} \dotp{f}{\meas} +  \sup_{\sup_\theta\norm{g(\theta)}_2  \leq \la_2} \dotp{g}{\meas}\\
&= \sup \enscond{ \dotp{f+g}{\meas} }{ \forall \theta, \; \norm{f(\theta)}_\infty \leq \la_1, \norm{g(\theta)}_2 \leq \la_2}
\end{split}
\end{equation}



%It is known from \cite{} that  for $\epsilon>0$,
%\begin{align*}
%&\enscond{x+y}{x,y\in\RR^d, \norm{x}_2 \leq \epsilon \nu, \norm{y}_\infty \leq (1-\epsilon) \nu} \\
%&= \enscond{\xi\in \RR^d}{\norm{\xi}_\epsilon \leq \nu}
%\end{align*}
%where the so-called $\epsilon$-norm, defined as $\nu = \norm{\xi}_\epsilon$  is the unique $\nu>0$ such that
%$$
%\sum_i (\abs{\xi_i} - (1-\epsilon)\nu)_+^2 - (\epsilon \nu)^2 = 0.
%$$
%Therefore,
From \eqref{eq:epsnorm1}, 
\begin{align*}
&\enscond{x+y\in\RR^d}{ \norm{x}_2 \leq \la_2 , \norm{y}_\infty \leq  \la_1 } \\
&= \enscond{\xi\in \RR^d}{ \norm{S_{\la_1}(\xi)}_2^2 \leq \la_2 }
\end{align*}
and
$
\norm{\meas}_{\beta} = 
\sup_{f\in\Kk_0}{\dotp{f}{\meas}}
$
where $$\Kk_0 = \enscond{ f\in \Cc(\Tspace;\RR^v)}{  \sup_{\theta\in\Tspace}   \norm{S_{\la_1}( f(\theta))}_2^2 \leq \la_2^2}.
$$
Note that we can restrict the set $\Kk_0$ to positive functions $\Kk_+ \eqdef \Kk_0 \cap \Cc(\Tspace;\RR_+^v)$ since $\meas$ is a positive measure.
Therefore, the convex conjugate of $J(\meas) \eqdef \norm{\meas}_\beta$ is $\iota_{\Kk_+}$, the indicator function on the set $\Kk_+$.

The result now follows by applying the Fenchel-Rockafellar duality theorem \cite[Thm 4.2]{ekeland1999convex}.

\end{proof}

Given a dual solution $Q_\alpha$ to \eqref{eq:spglassodual}, the function  $f(\theta) \eqdef \frac{1}{\la_2  }  (\eta(\theta) - \la_1)_+$ with $\eta \eqdef \Phi^* Q_\alpha$ characterizes the support of any primal solution $\meas_\alpha$ of \eqref{eq:spglasso} in the following sense:

\begin{lem}\label{lem:structure}
Any solution $\meas_\alpha$ to \eqref{eq:spglassodual} satisfies
$$
\Supp(\meas_\alpha) \subseteq \enscond{\theta\in\Tspace}{ \norm{f(\theta)} = 1  }.
$$
 If  $\meas_\alpha = \sum_s C_s^\top \delta(\theta - \theta_s)$ is a discrete measure, then for each $s$, $\Supp(C_s) \subseteq \enscond{j \in [v]}{\eta_j(\theta_s) > \la_1}$ and $f(\theta_s) = C_s/\norm{C_s}_2$.
 
 \end{lem}
\begin{proof}

We know $\eta = \Phi^* p \in \partial \abs{\meas}_\beta = \la_1 \partial \abs{\meas}_1  + \la_2 \abs{\meas}_2$.
From
\eqref{eq:eps_decomp}, if $\xi$ satisfies $\sum_i ( \xi - \la_1)_+^2 \leq \la_2^2$
then $\norm{S_{\la_1}(\xi)}_2 \leq \la_2$ and  $\norm{\xi - S_{\la_1}(\xi)}_\infty \leq \la_1$. So $S_{\la_1}(\eta) \in \la_2 \partial \abs{\meas}_2$ which gives the first inclusion. For the second,
$$
\eta - S_{\la_1} (\eta) \in \la_1 \partial \abs{\meas}_1
$$
which means that given $s\in [k]$ and $I_s = \Supp(C_s)$,
$$
\proj_{I_s } \pa{\eta(\theta_s) - \max(\eta(\theta_s) - \la_1 ,0) } = \la_1 \proj_{I_s} \sign(C_s)
$$
If  $ \eta(\theta_s)_j < \la_1 $ for $j\in I_s$, then this equation implies that $\eta(\theta_s)_j = \la_1 \sign(C_s)_j$ which is a contradiction. Therefore, $I_s \subset \enscond{j}{\eta_j(\theta_s)>\la_1}$.


\end{proof}



Note that \eqref{eq:spglassodual} has a unique solution, since it can be seen as the projection of $X/\alpha$ onto the closed convex set $K$.  Moreover, the previous lemma shows that its solution characterises the support of any primal solution $\meas$ of \eqref{eq:spglasso}. Therefore, to understand the structure of solutions to \eqref{eq:spglasso} with   $X = \Phi \meas + w$ with $\norm{w}\leq \epsilon$, it suffices to study the solution of the dual problem \eqref{eq:spglassodual}, which we denote by $Q_{\alpha,\epsilon}$.
%\begin{lem}
%Let $Q_\alpha$ solve \eqref{eq:spglassodual}. Then, letting $\eta_\alpha \eqdef \Phi^* p_\alpha$, any solution $\meas_\alpha$ to \eqref{eq:spglassodual} satisfies
%$$
%\Supp(\meas_\alpha) \subseteq \enscond{\theta\in\Tspace}{ \sum_i (\eta_i(\theta) - \beta)_+^2 =v (1-\beta)^2  }
%$$
% and if $\meas_\alpha = \sum_s C_s^\top \delta(\theta - \theta_s)$ is a discrete measure, then for each $s$, $\Supp(C_s) \subseteq \enscond{j \in [v]}{\eta_j(\theta_s) > \beta}$.
%\end{lem}
Following \cite{duval2015exact}, we can show that $Q_{\alpha,\epsilon}$ has a limit as $\epsilon/\alpha$ and $\alpha$ converge to 0:
Define the \textit{minimal norm certificate} by
\begin{equation}
\begin{split}
Q_0 \in \argmin \enscond{\norm{Q}_F}{\eta \eqdef \Phi^* Q \in \Kk, \; \dotp{\eta}{\meas} = \norm{\meas}_\beta}.
\end{split}
\end{equation}
\begin{lem}
We have $\norm{Q_{\alpha,0} - Q_0}_F \to 0$ as $\alpha\to 0$, and
$$
\norm{Q_{\alpha,\epsilon} - Q_{\alpha, 0}}_F \leq \epsilon/\alpha.
$$
\end{lem}
\begin{proof}
The proof is omitted as it is verbatim the proof of Proposition \ref{} in \cite{duval2015exact}
\end{proof}

\begin{rem}
The minimal norm certificate $Q_0$ is  a solution to the dual problem \eqref{eq:spglassodual} with $\alpha = 0$ and $X = \Phi \meas$. Moreover, from Lemma \ref{lem:structure}, for a discrete measure $\meas = \sum_s C_s^\top \delta_{\theta_s}$, we in fact have, writing $f_Q \eqdef\frac{1}{\la_2}(\Phi^* Q - \la_1)_+$,
\begin{equation}
\begin{split}
Q_0 \in \argmin \enscond{\norm{Q}_F}{  \sup_{\theta\in\Tspace} \norm{f_Q(\theta)}_2 \leq 1 \;f_Q(\theta_s) = \frac{C_s}{\norm{C_s}_2}}.
\end{split}
\end{equation}
\end{rem}

Define $\eta_0 \eqdef \Phi^* Q_0$  and $f_0 \eqdef \frac{1}{\la_2} (\eta_0 -\la_1)_+$.
We say that $Q_0$ is nondegenerate  with respect to a sparse measure $\mestar = \sum_{s=1}^k C_s \delta(\theta - \theta_s)$ 
satisfies 
\begin{enumerate}
\item $\norm{f_0(\theta)}_2<1$ for all $\theta\not\in \ens{\theta_i}$
\item for each $s\in [k]$, $f_0(\theta_s) =  \frac{C_s}{\norm{C_s}_2}$.
\item  letting $g(\theta) \eqdef  \norm{f_0(\theta)}_2^2$, $g''(\theta_s) \neq 0$ for all $s\in [k]$. 
%and 
%$$
%\sum_{i\in \Supp(C_s)} ({\eta_i(\theta_s)} - \beta )_+\nabla^2 \eta_i(\theta) +\nabla \eta_i(\theta_s) [\nabla \eta_i(\theta_s) ]^\top <0
%$$
\end{enumerate}

\begin{prop}\label{prop:stability}
If $Q_0$ is nondegenerate, then provided that $\epsilon/\alpha$ and $\alpha$ are sufficiently small, the solution to \eqref{eq:spglasso} is of the form $\meas_{\alpha,\epsilon} = \sum_{j=1}^k \hat C_j \delta_{\hat \theta_j}$ where $\Supp(\hat C_j) \subseteq \Supp(C_j)$.
\end{prop}
\begin{proof}
From \eqref{eq:spglassodual}, we see that the dual solution to \eqref{eq:spglassodual} can be written as the projection of $X/\alpha$ onto the set $\Kk$. 
So, from $\norm{Q_{\alpha,\epsilon}-Q_{\alpha,0}} \leq  \norm{\proj_\Kk(X/\alpha) - \proj_\Kk((X+w)/\alpha)}  \leq \norm{w}_F/\alpha$, we have that $\eta_{\al,\epsilon} \eqdef \Phi^* Q_{\al,\epsilon} \to \eta_0$ in the uniform norm as $\alpha$ and $\epsilon/\alpha$ converge to 0. So, if $\eta_0$ is non-degenerate, then given any $r>0$, provided that $\norm{w}_F/\alpha$ and $\alpha$ are sufficiently small, letting $g(\theta) \eqdef \frac{1}{\la_2^2} \norm{(\eta_{\al,\epsilon}(\theta) - \la_1)_+}^2 $, we have $g(\theta)<1$ for all $\theta \not\in  \cup_j \Bb(\theta_j,r)$, and for all $\theta\in \Bb(\theta_j,r)$, $g''(\theta) \neq 0$. So, there are at most $k$ points for which $g(\theta) = 1$.  So, by Lemma \ref{lem:structure}, given data $X =\Phi \meas + w$, we recover at most $k$ components with $\meas_{\alpha,\epsilon} = \sum_{j=1}^k \hat C_j \delta_{\hat \theta_j}$. Finally, uniform convergence of $\eta_{\alpha,\epsilon}$  to $\eta_0$ also ensures that $\Supp(\hat C_j) \subseteq \Supp(C_j)$ for $\alpha$ and $\epsilon/\alpha$ sufficiently small.
\end{proof}


To establish support stability, it suffices to show that $Q_0$ is nondegenerate. 
In general, $Q_0$ does not have a closed form expression and can be hard to compute, and in practice, one computes the precertificate $Q_V$ instead: Notice that
since $\norm{f_0(\theta)}^2 \leq 1$ for all $\theta$ and $\norm{f_0(\theta_s)}_2 = 1$, it is necessary that $\partial_\theta \norm{f_0(\theta_s)}_2^2 = 0$  for all $s\in [k]$. Hence, if we add the constraint that $\sup_\theta \norm{ f_p(\theta)}\leq 1$ to the constraint set in the definition of the vanishing derivatives precertificate $\eta_V$, then we have $\eta_V = \eta_0$. In other words, if  $\sup_\theta \norm{ f_V(\theta)}\leq 1$, then we must have $\eta_V = \eta_0$, and moreover, nondegeneracy of $\eta_V$ implies  that $\eta_0 = \eta_V$ is also nondegenerate.




%We look at the following proxy of $Q_0$ which has a closed form expression: Let  $s\in [k]$ and $I_s \eqdef \Supp(C_s)$. First note that the constraint $f_0(\theta_s) = \frac{C_s}{\norm{C_s}_2}$ can be written as
%\begin{align*}
%\proj_{\bold{I}} \vc\pa{ \Phi^\top_{\btheta} Q_0}= \proj_{\bold{I}} [\Id_v \otimes D_{\btheta}^\top]\vc(Q_0) = u_0
%\end{align*}
%where $u_0 = \pa{\beta + \sqrt{v}(1-\beta) \proj_{I_s}  C_s/\norm{C_s}_2}_{s=1}^k \in \RR^{\sum_s \abs{I_s}}$ and given $Z=(Z_s)_{s=1}^k \in \RR^{k v}$, $\proj_{\bold{I}}(Z) =( \proj_{I_s} Z_s)_{s=1}^k$. Since $\norm{f_0(\theta)}^2 \leq 1$ for all $\theta$ and $\norm{f_0(\theta_s)}_2 = 1$, it is necessary that $\partial_\theta \norm{f_0(\theta_s)}_2^2 = 0$  for all $s\in [k]$, and hence,
%\begin{align*}
%\mathbf{0}_d &= \sum_{i=1}^v (C_s)_i \nabla (\eta_0)_i(\theta_s) \\
%&= \JJ_\phi(\theta_s)^\top Q_0 C_s =[ C_s^\top\otimes \JJ_\phi(\theta_s)^\top]\vc(Q_0)
%\end{align*}
%Defining the $Tv\times (\sum_{s=1}^k \abs{I_s}+kd)$ matrix $$
%\Gamma = \left[(\Id_v\otimes D_\btheta ) \proj_{\bold{I}}^* , C_1\otimes \JJ_\phi(\theta_1), \cdots, C_k \otimes \JJ_\phi(\theta_k) \right]
% $$
%we see that $Q_0$ must satisfy
%$$
%\Gamma^{*} Q_0 = \begin{pmatrix}
%u_0\\
%\mathbf{0}_{kd}
%\end{pmatrix}.
%$$
%So, if $\eta_V \eqdef \Phi^* \rc \pa{(\Gamma^*)^\dagger \begin{pmatrix}
%u_0\\
%\mathbf{0}_{kd}
%\end{pmatrix}}$ satisfies $\norm{S_\beta(\eta_V(\theta))}_2 \leq \sqrt{v}(1-\beta)$ for all $\theta$, then $\eta_V = \eta_0$ and we have a closed form expression for $\eta_0$.  

%Define $f_V(\theta)  \eqdef \frac{1}{\sqrt{v}(1-\beta)}(\eta_V(\theta) - \beta)_+$. Note that by definition, $f_V(\theta_s) = f_0(\theta_s)$. 
%\begin{defn}
%We call  $\eta_V$ the vanishing derivatives precertificate and say that it is nondegenerate if $f_V(\theta) <1$ for all $\theta \not\in \ens{\theta_s}_{s=1}^k$ and $ g_V(\theta) \eqdef  \norm{f_V(\theta)}^2$ satisfies $g_V''(\theta_s) \neq 0$ for all $s\in [k]$.
%
%\end{defn}
%Clearly, if $\eta_V$ is nondegenerate, then $\eta_V = \eta_0$ is also nondegenerate.
\subsection{Proof of Theorem \ref{thm:stability}}\label{supp:theory_proof}


%\begin{thm}\label{thm:stability}
%Let $X = \Phi \mestar + \epsilon$ where $\epsilon \in \RR^{T\times v}$ satisfies $\norm{\epsilon}_F \leq \delta$ and $\mestar = \sum_{s=1}^k C_s \delta_{\theta_s}$. Suppose that $\Gamma$ is full rank and $\eta_0 \eqdef \Phi^* Q_0$ is nondegenerate, then for all $\alpha$ and $\delta/\alpha$ sufficiently small,  \eqref{eq:spglasso} recovers a unique solution of the form $ \sum_{s=1}^k \tilde C_s \delta(\theta - \tilde \theta_s)$ with $\norm{\tilde C_s - C_s}_F \leq \delta$ and $\norm{\tilde \theta_s - \theta_s} \leq \delta$.
%
%\end{thm}





\begin{proof}[Proof of Theorem \ref{thm:stability}]


Let $\mestar =  \sum_s (C^*_s)^\top {\delta}_{\theta^*_s}$.
We already know from Proposition \ref{prop:stability} that for small $\alpha$ and $\epsilon/\alpha$, the support of  $\meas_{\alpha,\epsilon}$ has the same cardinality as as that of $\mestar$ and can be made arbitrarily close to $\Supp(\mestar)$. To obtain the required error bound, we exploit the implicit function theorem.

 


Define a function
$$
F:\RR_+^{\sum_s \abs{I_s}} \times \Tspace^k \times \RR^{T \times v}\times  \RR_+ \to \RR^{\sum_{s=1}^k \abs{I_s} + kd}
$$
by $F(C,\btheta,W,\alpha) = \begin{bmatrix}
\pa{g_i(C,\btheta,W,\alpha)}_{i=1}^k\\
\pa{h_i(C,\btheta,W,\alpha)}_{i=1}^k
\end{bmatrix}$
where writing $x\eqdef (C,\btheta,W,\alpha)$,
$$
g_s(x) = \proj_{I_s}
\pa{ \phi(\theta_s)^\top[D_\btheta \bar C^\top -D_{\btheta^*} (C^*)^\top - w ] }+ \alpha \pa{ \lambda_1 +  \lambda_2 \frac{C_s^\top}{\norm{C_s}}}
$$
and
$$
h_s(x) = J_{\phi}(\theta_s)^\top \pa{D_\btheta \bar C^\top - D_{\btheta^*} (C^*)^\top - W} \frac{C_s}{\norm{C_s}_2}.
$$
Here, $\bar C \in \RR^{ v\times k}$ is the matrix with $s^{th}$ column satisfying  $(\bar C_s)_{I_s} = C_s$ and $(\bar C_s)_{I_s^c} = 0$.
Clearly, if $(C,\btheta)$ correspond to a solution with data $y= D_{\btheta^*} (C^*)^\top + W$, then $F(C,\btheta,W,\alpha) = 0$. Note also that $F(C^*, \btheta^*, 0,0) = 0$.



Writing $x = (C,\btheta)$, $N= \sum_{s}\abs{I_s}$, $$\partial_x F(C^*,\btheta^*,0,0) = \Gamma_{\btheta^*,C^*}^\top \Gamma_{\btheta^*,C^*} \begin{pmatrix}
\Id_{N} & \mathbf{0}_{N \times kd}\\
\mathbf{0}_{kd\times N } &\diag\pa{\norm{C_s}_2}_{s=1}^k \otimes \Id_{d}
\end{pmatrix}
$$
By assumption, $\partial_x F$ is invertible. By the implicit function theorem, there exists neighbourhoods $\Xx \subset \RR_+^{kv} \times \Tspace^k$ of $(C^*, \btheta^*)$ and $\Yy \subset \RR^{Lv}\times \RR_+$ of $(0,0)$ and a unique  continuously differentiable function $g:\Yy \to \Xx$ such that $F(g(y), y) = 0$ for all $y = (W,\alpha)\in V$. Moreover, since $g$ is continuously differentiable, $\norm{g(y) - g(0)} \leq C \norm{y}$. In particular, writing $(C,\btheta) = g(y)$,
$$
\norm{C - C^*}_F+ \norm{\btheta - \btheta^*} \leq C (\alpha + \norm{W}_F) .
$$
Finally,  since we have already established support stability in Proposition \ref{prop:stability}, by uniqueness, $g(y)$ coincides with solutions of \eqref{eq:spglasso}.


\end{proof}


\section{Derivation of Algorithm \ref{alg:FW}}

%%%%%%%%%%%%%%%%%%%%%
We follow the presentation of \cite{denoyelle2019sliding} where the sliding Frank-Wolfe was presented for scalar-valued measures.
The Frank-Wolfe algorithm seeks to solve minimisation problems of the form 
$$
\min_{m\in \Kk} F(m)
$$
where $f:\Xx\to \RR$ is a continuously differentiable function defined on some Banach space $\Xx$, and $\Kk \subseteq \Xx$ is a bounded convex  set. To  derive our algorithm, we follow \cite{denoyelle2019sliding} by rewriting \eqref{eq:spglasso} as the minimisation of a differentiable function over a bounded convex set. Note that  the optimal measure satisfies
$$
\frac12 \norm{\Phi \meas - X}_F^2 +  \alpha \norm{\meas}_\beta  \leq \norm{X}_F^2/2
$$
Recalling the definition of $\norm{\cdot}_\beta$, we can write $ \alpha \norm{\meas}_\beta  = \lambda_1 \abs{\meas}_1+ \lambda_2 \abs{\meas}_2$ where $\lambda_1 = \alpha (1-\beta)$ and $\lambda_2 = \alpha \beta \sqrt{v}$.
So in particular, $\abs{\meas}_{1} \leq \norm{X}_F^2/\pa{2\lambda_1}$. We can therefore equivalently write this as
\begin{align*}
\min_{\meas\in\Mm_+(\Tspace;\RR^p), t_1,t_2\in\RR} F(t_1,t_2,\meas) \eqdef \lambda_1 t_1 + \lambda_2 t_2 + \frac12 \norm{\Phi\meas - y}^2
\\
\qquad \text{subject to } (t_1,t_2,\meas)\in \Kk
\end{align*}
where $\Kk\eqdef \enscond{(t_1,t_2,\meas)}{\abs{\meas}_1 \leq t_1,  \abs{\meas}_{2}\le t_2,  t_2 \leq t_1 \leq \frac{\norm{X}_F^2}{2\lambda_1}}$.
The differential of $F$ is a bounded linear operator on $\RR\times \RR \times \Mm_+(\Tspace;\RR^p)$. Writing $s \eqdef (t_1,t_2,\meas)$ and $s' \eqdef (t_1',t_2',\meas')$, we have  
$$
[\mathrm{d}F(s)]s' = \lambda_1 t_1' + \lambda_2 t_2' + \int [\Phi^*( \Phi \meas - y)] (\theta) \mathrm{d}\meas'(\theta)
$$
The Frank-Wolfe algorithm is an iterative algorithm consisting of the following two steps: Denoting the $k$th iterate by $x^k$, do
\begin{enumerate}
\item $
s^{k} \in \argmin_{s\in\Kk} \mathrm{d}F(x^k)(s)
$
\item $x^{k+1} = (1-\gamma_k) s^{k} +\gamma_k x_k$
\end{enumerate}
For the first step, we can restrict the minimisation to the the extremal points of the convex set $\Kk$, which are of the form $(\norm{M}_1, \norm{M}_2, M \delta_\theta)$ where $\theta\in \Tspace$ and $M\in \RR_+^v$. Therefore, writing $x^k = (t_1,t_2,\meas^k)$, we are led to solve
\begin{equation}\label{eq:tosolve}
(\theta,M) \in \argmin_{\theta\in\Tspace, M\in \RR^p_+}   \lambda_1 \norm{M}_1 + \lambda_2 \norm{M}_2 - \dotp{M}{\eta^k(\theta) }, 
\end{equation}
where $ \eta^k\eqdef -\Phi^*( \Phi \meas^k - y)$.
Let the optimal points be $M = (m_j)_{j=1}^v$ and $\theta$, then the optimality condition reads
$$
-\eta^k(\theta)_j + \lambda_2 \frac{m_j}{\norm{M}_2} + \lambda_1 = 0, \qquad \text{ if } m_j >0
$$
$$
\eta^k(\theta)_j \in [0, \lambda_1], \qquad \text{ if } m_j =0
$$
i.e. we have 
$$
  \frac{M}{\norm{M}_2} = \frac{1}{\lambda_2} \pa{  \eta^k(\theta) - \lambda_1}_+
$$
Plugging this back into \eqref{eq:tosolve} and simplifying, we are left with
\begin{align}
\theta \in  \argmax_{\theta\in\Tspace} 
     \sum_{i=1}^p \pa{  \eta^k(\theta)_i - \lambda_1}_+^2
\end{align}
The second step of the algorithm can be replaced by any procedure which improves the objective value, which leads to the optimization problems in lines 8 and 9 of Algorithm \ref{alg:FW}.
